# Supplementary material for: BiFSMN: Binary Neural Network for Keyword Spotting
Source: arXiv:2202.06483 source file (2022-10-20)
Supplement: Supplementary file 1 [file supp.tex]

\subsection{Binarization Framework}
First of all, we build a comprehensive binarized KWS baseline including various model architectures (i.e. VGG-16, BCResNet, FSMN) with several representative and efficient binarization practice. We brief each technique in the following: % bnn bwn（vanilla） xnor ir-net bireal loss-aware
\textbf{Binarized-Neural-Networks (BNN).} As a representative, BNN binarzes both weights and activations to 1-bit using $\mathtt{sign}$ function in the forward and $\mathtt{Hardtanh}$ to clip the gradient, which can be formulated as follows:
\begin{equation}
\begin{aligned}
\label{eq:bnn}
%Q(\mathbf X)=\alpha\mathbf{B} ,\quad 
&\mathrm{Forward:}\ b=\mathtt{sign}(x)=
\begin{cases}
+1,& \mathrm{if} \ x \ge 0\\
-1,& \mathrm{otherwise}
\end{cases}, \\
%\mathrm{Backward:}\ g_{x}=g_{b} {1}_{|x| \leq 1},
% &\mathrm{Backward:}\ g_{x}=
% \begin{cases}
% g_b,& \mathrm{if} \ x \in \left(-1, 1\right)\\
% 0,& \mathrm{otherwise} 
&\mathrm{Backward:}\ g(x) = \mathtt{Hardtanh}(x) = \mathtt{max}(-1, \mathtt{min}(1, x)), % \mathtt{Clip}(x, -1,1)
% \end{cases}
\nonumber
\end{aligned}
\end{equation}
where $x$ denotes the element in floating-point weights $\mathbf{w}$ and activations $\mathbf{a}$, $b$ denotes the element in binarized weights $\mathbf{B_w}$ and activations $\mathbf{B_a}$. %$g_{x}$, and $g_{b}$ donate the gradient $\frac{\partial C}{\partial x}$ and $\frac{\partial C}{\partial b}$, respectively, where $C$ is the cost function for the minibatch.
    
\textbf{Binary-Weight-Networks (BWN). } Full-precision scaling factor $\alpha$ is introduced to retain the magnitude of real-value weights:
\begin{equation}
\label{eq:bwn}
\alpha^* = \frac{\mathbf{w}^\top \mathtt{sign} (\mathbf{w})}{n} = \frac{1}{n} \left\| \mathbf{w} \right\|_{l1},
\nonumber
\end{equation}
we make $\mathbf{w} \approx \alpha \mathbf{B_w}$ to reduce the quantization error.
    
\textbf{XNOR-Networks (XNOR-Net).} It employs learnable weight scalar $\alpha$ and activation scalar $\beta$ so as to approximate the original full-precision dot product, i.e. $\mathbf{a^\top} \mathbf{w} \approx \beta \mathbf{B_a ^ \top} \alpha \mathbf{B_w}$. 
% $\beta, \alpha \in \mathbb{R}^+$ are learnable with an objective function:
% \begin{equation}
%     \alpha^*, \mathbf{B_a}^*, \beta^*, \mathbf{B_w}^* = \argmin_{\alpha, \mathbf{B_a}, \beta, \mathbf{B_w}} \left \| \mathbf{A} \odot \mathbf{W} - \beta\alpha \mathbf{B_w} \odot \mathbf{B_a} \right \|
%     \nonumber
% \end{equation}
% where $\odot$ indicates element-wise product. In this way, quantization error was minimized. 
    
\textbf{Information Retention Network (IR-Net). } It uses standardized balanced weights to get binarized ones to mitigate the negative effect of weight magnitude, and an approximation of backward gradient:
\begin{equation}
\begin{aligned}
\label{eq:ir-net}
&\mathrm{Forward:}\ \mathbf{w}_{std} = \hat{\mathbf{w}} / \sigma (\mathbf{w}), \ \hat{\mathbf{w}} = \mathbf{w} - \bar{\mathbf{w}}, \\
&\mathrm{Backward:}\ g(x) = k\ \mathtt{tanh}\ tx , 
\nonumber
\end{aligned}
\end{equation}
where $\sigma (\cdot)$ denotes the standard deviation, $t, k$ are control variables varying according to the training process. 
    
\textbf{Bi-Real Net. } It utilizes a piecewise polynomial function to approximate the sign function for binarizing activations, and multiple weight magnitude to $\mathtt{sign}$ function for precise gradient in backpropagation. 
% \begin{equation}
% \begin{aligned}
%     \label{eq:bireal-net}
%     &\mathrm{Forward:}\ b_a = 
%     \begin{cases}
%     -1 & \mathrm{if}\ a < -1 \\
%     2a+a^2 & \mathrm{if}\ -1 \le a < 0 \\
%     2a - a^2 & \mathrm{if}\  0 \le a < 1 \\
%     1 & \mathrm{otherwise} 
%     \end{cases}, \\ 
%     &\mathrm{Backward:}\ \frac{\delta b_a}{a} = 
%     \begin{cases}
%     2 + 2a & \mathrm{if}\ -1 \le a < 0 \\
%     2 - 2a & \mathrm{if}\ 0 \le a < 1 \\
%     0 & \mathrm{otherwise} 
%     \end{cases},
%     \nonumber
% \end{aligned}
% \end{equation}
% where $b_a$ denotes the element in $\mathbf{B_a}$, and $a$ denotes the element in full-precision activations $\mathbf{a}$.
    
\textbf{Loss-aware training.} Previous work \cite{} proposes three loss functions while training the quantized model for solving the degeneration, saturation, gradient mismatch problems, respectively. 

Though many advanced techniques have been proposed in binarization, the models we obtain in the baseline still suffer severe accuracy drop. 
\dyf{TODO: loss landscape...}

\subsection{BiFSMN}
With the challenge of limited representation capability and difficulty in training 1-bit parameters, we propose a novel binarized FSMN, dubbed BiFSMN. 

\subsubsection{Outline Distillation via Wavelet Transform}
\subsubsection{Building a Slim BiFSMN}
\subsubsection{Efficient Deployment}
